# Supplementary material for: CubeFormer: A Simple yet Effective Baseline for Lightweight Image Super-Resolution
Source: arXiv:2412.02234 source file (2024-12-03)
Supplement: Supplementary file 1 [file X_suppl.tex]

\clearpage
\setcounter{page}{1}
\maketitlesupplementary

%\section{Rationale}
%\label{sec:rationale}
% 
%Having the supplementary compiled together with the main paper means that:
% 
%\begin{itemize}
%\item The supplementary can back-reference sections of the main paper, for example, we can refer to \cref{sec:intro};
%\item The main paper can forward reference sub-sections within the supplementary explicitly (e.g. referring to a particular experiment); 
%\item When submitted to arXiv, the supplementary will already included at the end of the paper.
%\end{itemize}
% 
%To split the supplementary pages from the main paper, you can use \href{https://support.apple.com/en-ca/guide/preview/prvw11793/mac#:~:text=Delete%20a%20page%20from%20a,or%20choose%20Edit%20%3E%20Delete).}{Preview (on macOS)}, \href{https://www.adobe.com/acrobat/how-to/delete-pages-from-pdf.html#:~:text=Choose%20%E2%80%9CTools%E2%80%9D%20%3E%20%E2%80%9COrganize,or%20pages%20from%20the%20file.}{Adobe Acrobat} (on all OSs), as well as \href{https://superuser.com/questions/517986/is-it-possible-to-delete-some-pages-of-a-pdf-document}{command line tools}.

%\section{Detailed Quantitative Comparison}
%
%We have reported PSNR and SSIM comparison in our paper with several state-of-the-art methods 
%
%
\begin{figure*}[hb]
    \centering
    \includegraphics[width=1.0 \linewidth, trim=0 350 180 0, clip]{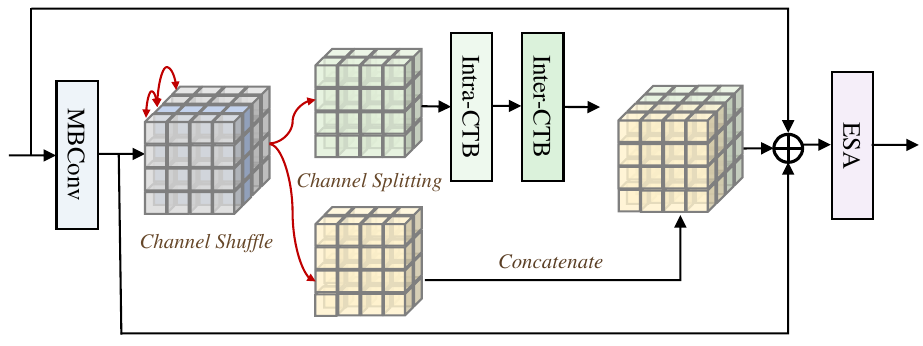}
    %\includesvg[width=\linewidth]{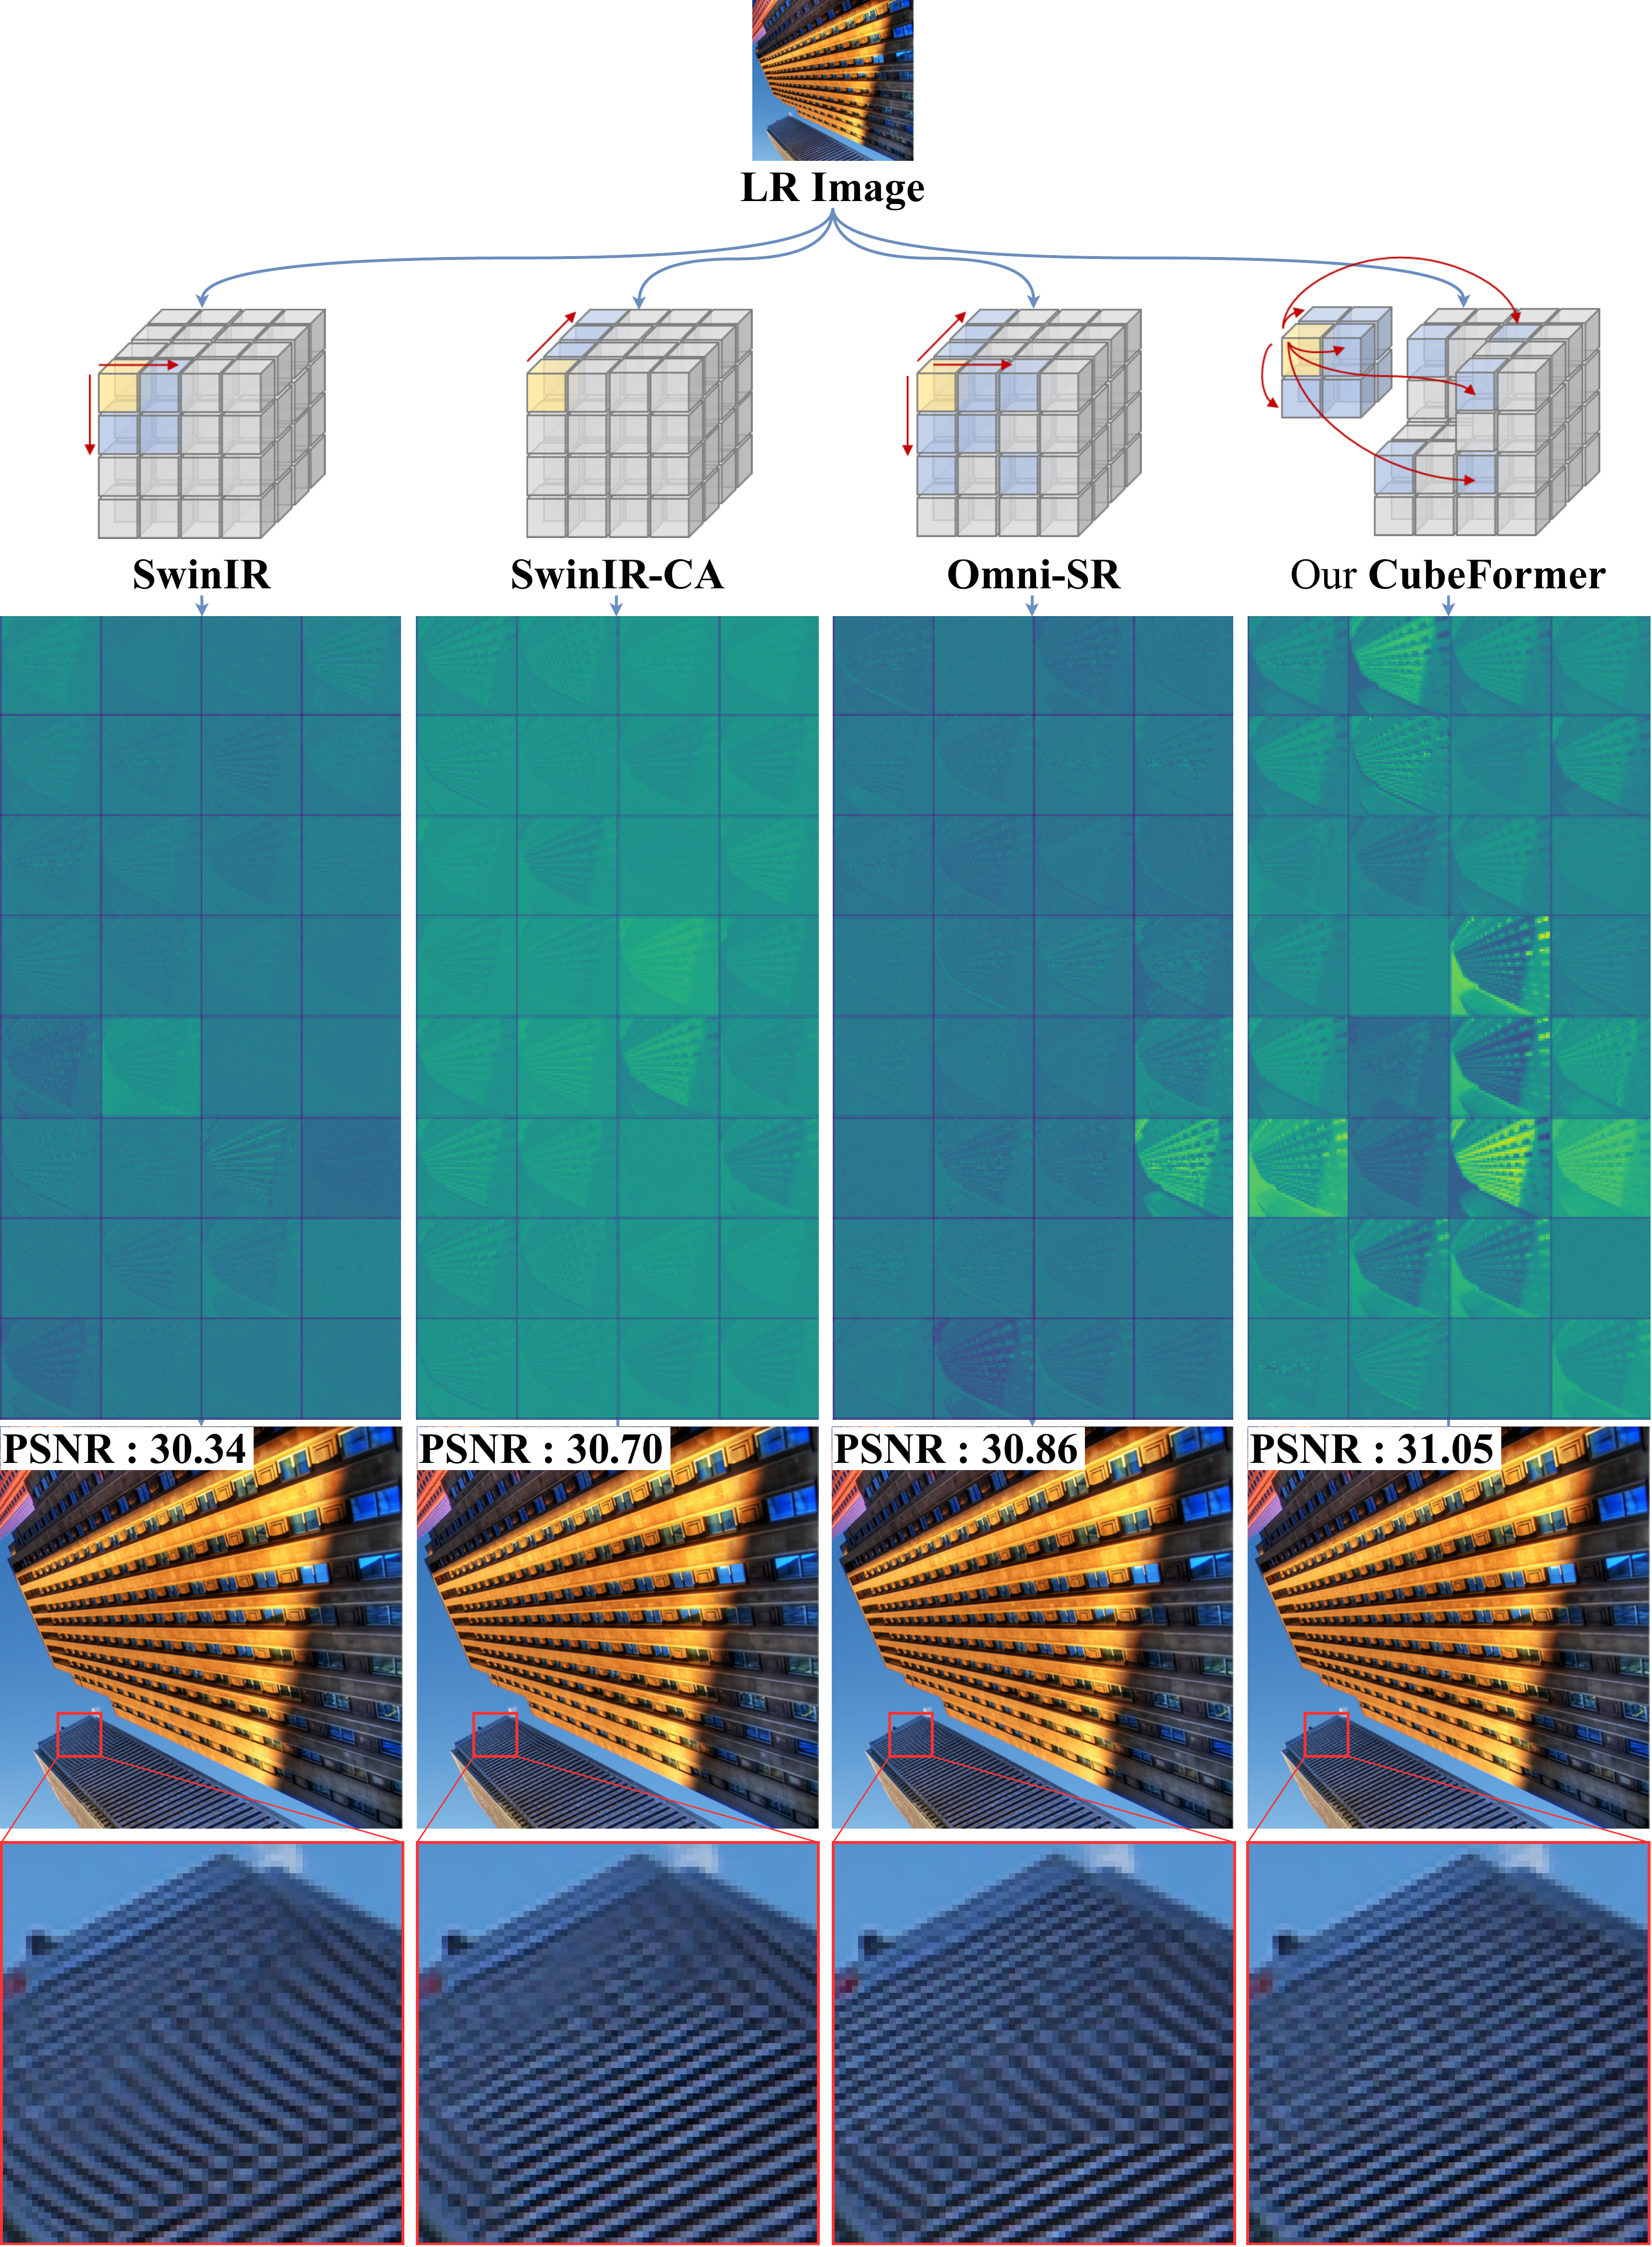}
    \caption{
    Illustration of Cube Transformer Group (CTG) and its lightweight version, CTG-lite. In CTG-lite, an additional channel split operation is introduced after the channel shuffle to partition the features into two groups with halved channels. Only one group participates in the subsequent computations and is then concatenated with the other group to form the features for residual addition and the Enhanced Spatial Attention (ESA) operation.
    }
    \vspace{-6mm}
    \label{fig:ctg_lite}
\end{figure*}

\section{CubeFormer-lite}
In our paper, we have mentioned a lite version of our proposed CubeFormer for efficient super-resolution, CubeFormer-lite.
It significantly reduces the number of network parameters while maintaining competitive performance.
To constitute CubeFormer-lite, we streamline the Cube Transformer Group (CTG) of the CubeFormer, which is renamed as CTG-lite.

\textbf{Channel split}.
As illustrated in Figure \ref{fig:ctg_lite}, in CTG-lite, we add an additional channel split operation \cite{ma2018shufflenet} after the channel shuffle operation \cite{zhang2018shufflenet} to divide the features into two equal groups in the channel dimension.
One group participates in the next operations of intra-CTB and inter-CTB, while the other group skips these calculations and is concatenated with the calculated first group.
This reduction in the involvement of features allows us to decrease the intra-CTB and inter-CTB parameters, which constitute the majority of the overall model parameters.
\\ \indent
\textbf{CTG-lite}.
Suppose the input feature of CTG-lite is $X_{in} \in \mathbb{R}^{H\times W\times C}$.
It first passes through the MBConv block \cite{howard2017mobilenets, hu2018squeeze}, and then conducts channel shuffle and channel split, where the input feature $X_{in}$ is separated into two parts: $X_{1} \in \mathbb{R}^{H\times W\times \frac{C}{2}}$ and $X_{2} \in \mathbb{R}^{H\times W\times \frac{C}{2}}$.
This process can be described by the following equation:
\begin{equation}
    X_{1}, X_{2} = Split(Shuffle(H_{MB}(X_{in}))),
\end{equation}
where $Split(\cdot)$ and $Shuffle(\cdot)$ refer to the channel split operation and channel shuffle operation. 
$H_{MB}(\cdot)$ denotes the transformation of the MBConv block.
We suppose that $X_{1}$ is for the next operations, and $X_{2}$ skips these computations and is directly concatenated after the operated $\hat{X_{1}}$ for generating $\hat{X}$.
$\hat{X}$ is the input of the following enhanced spatial attention (ESA) module \cite{liu2020residual} to get the output features $X_{out}$.
This stage can be represented by the equations below:
\begin{equation}
\begin{aligned}
    &\hat{X_{1}} = H_{inter}(H_{intra}(X_{1})), \\
    &\hat{X} = Concat(\hat{X_{1}}, X_{2}), \\
    &X_{out} = H_{ESA}(\hat{X}), \\
\end{aligned}
\end{equation}
where $H_{intra}(\cdot)$ and $H_{inter}(\cdot)$ denote the transformation of intra-CTB and inter-CTB, $H_{ESA}(\cdot)$ represents the ESA module's transformation, and $Concat(\cdot, \cdot)$ refers to the channel concatenation operation.
%
%\\ \indent
